# Supplementary material for: Low-Quality Training Data Only? A Robust Framework for Detecting Encrypted Malicious Network Traffic
Source: arXiv:2309.04798 source file (2023-09-09)
Supplement: Supplementary file 1 [file appendix_real_dataset.tex]

\begin{table*}[ht]
    \centering
    \caption{F1-score of each detection model on Private Dataset}
    \label{tab:detection_f1}
    \resizebox{\textwidth}{!}{
        \begin{tabular}{c|c|c|cccccc|cc}
            \toprule
            \multirow{2}{*}{\textbf{Quantity}} & \multirow{2}{*}{\textbf{Noise Ratio}} & \multicolumn{9}{c}{\textbf{Detection Methods}} \\
             & & \textbf{Our Method} & FS & Co+FS & DT+FS & ODDS+FS & SMOTE+FS & DT+ODDS+FS & ETA & DT+ODDS+ETA\\
            \midrule \midrule
            \multirow{6}{*}{250} 
             & 20\% & 0.602 & 0.150 & 0.001 & 0.394 & 0.366 & 0.444 & 0.158 & 0.615 & 0.617 \\
             & 25\% & 0.653 & 0.294 & 0.001 & 0.152 & 0.096 & 0.367 & 0.153 & 0.376 & 0.376 \\
             & 30\% & 0.630 & 0.403 & 0.005 & 0.270 & 0.070 & 0.401 & 0.123 & 0.433 & 0.351 \\
             & 35\% & 0.541 & 0.314 & 0.083 & 0.352 & 0.201 & 0.356 & 0.276 & 0.291 & 0.202 \\
             & 40\% & 0.555 & 0.128 & 0.223 & 0.243 & 0.153 & 0.322 & 0.363 & 0.370 & 0.322 \\
             & 45\% & 0.614 & 0.321 & 0.368 & 0.468 & 0.209 & 0.346 & 0.167 & 0.218 & 0.225 \\
            \midrule
            \multirow{6}{*}{500} 
             & 20\% & 0.583 & 0.198 & 0.001 & 0.407 & 0.221 & 0.339 & 0.460 & 0.381 & 0.382 \\
             & 25\% & 0.642 & 0.224 & 0.181 & 0.295 & 0.205 & 0.300 & 0.335 & 0.575 & 0.559 \\
             & 30\% & 0.655 & 0.064 & 0.081 & 0.239 & 0.150 & 0.318 & 0.155 & 0.596 & 0.447 \\ 
             & 35\% & 0.527 & 0.261 & 0.164 & 0.414 & 0.237 & 0.330 & 0.271 & 0.413 & 0.318 \\
             & 40\% & 0.574 & 0.330 & 0.143 & 0.257 & 0.057 & 0.294 & 0.033 & 0.464 & 0.417 \\
             & 45\% & 0.619 & 0.271 & 0.261 & 0.349 & 0.180 & 0.310 & 0.469 & 0.054 & 0.075 \\
             \midrule
            \multirow{6}{*}{1000} 
             & 20\% & 0.610 & 0.252 & 0.009 & 0.393 & 0.264 & 0.311 & 0.107 & 0.583 & 0.552 \\
             & 25\% & 0.627 & 0.464 & 0.001 & 0.460 & 0.165 & 0.308 & 0.289 & 0.370 & 0.442 \\
             & 30\% & 0.601 & 0.222 & 0.247 & 0.276 & 0.300 & 0.291 & 0.071 & 0.479 & 0.516 \\
             & 35\% & 0.584 & 0.293 & 0.333 & 0.391 & 0.280 & 0.292 & 0.028 & 0.301 & 0.265 \\
             & 40\% & 0.600 & 0.273 & 0.123 & 0.368 & 0.311 & 0.289 & 0.373 & 0.228 & 0.265 \\
             & 45\% & 0.634 & 0.394 & 0.119 & 0.194 & 0.106 & 0.298 & 0.194 & 0.311 & 0.233 \\
            \bottomrule
        \end{tabular}
    }
\end{table*}

\begin{table}[ht]
    \centering
    \caption{Detection performance after data augmentation}
    \label{tab:data-augmentation-results}
    \resizebox{\columnwidth}{!}{
        \begin{tabular}{|c|c|r|r|r|}
            \cline{1-5}
            \textbf{Quantity} & \textbf{Method} & F1-score & Recall & Precision\\
            \cline{1-5}
            \multirow{4}{*}{250} & \textbf{Our Method} & 0.620 & 0.898 & 0.474 \\ 
            \cline{2-5}
             & ODDS & 0.230 & 0.183 & 0.221 \\ 
            \cline{2-5}
             & SMOTE & 0.260 & 0.221 & 0.550 \\
            \cline{2-5}
             & GAN & 0.385 & 0.326 & 0.497 \\
            \cline{1-5}
            \multirow{4}{*}{500} & \textbf{Our Method} & 0.707 & 0.804 & 0.637 \\ 
            \cline{2-5}
             & ODDS & 0.053 & 0.030 & 0.310 \\ 
            \cline{2-5}
             & SMOTE & 0.247 & 0.165 & 0.642 \\
            \cline{2-5}
             & GAN & 0.316 & 0.278 & 0.596 \\
            \cline{1-5}
            \multirow{4}{*}{1000} & \textbf{Our Method} & 0.709 & 0.792 & 0.659 \\ 
            \cline{2-5}
             & ODDS & 0.090 & 0.049 & 0.665 \\ 
            \cline{2-5}
             & SMOTE & 0.576 & 0.571 & 0.649 \\
            \cline{2-5}
             & GAN & 0.415 & 0.388 & 0.535 \\
            \cline{1-5}
        \end{tabular}
    }
\end{table}
