# Supplementary material for: Low-Quality Training Data Only? A Robust Framework for Detecting Encrypted Malicious Network Traffic
Source: arXiv:2309.04798 source file (2023-09-09)
Supplement: Supplementary file 2 [file little_noise_appendix.tex]

\begin{table*}[ht]
    \centering
    \caption{The F1-score with few-noise training set}
    \label{tab:detection_f1_little_noise}
    \resizebox{0.9\textwidth}{!}{
        \begin{tabular}{c|c|cccccc|cc|c}
            \toprule
            \multirow{2}{*}{\makecell[c]{\textbf{Noise} \\ \textbf{Ratio}}} & \multirow{2}{*}{\textbf{Dataset}} & \multicolumn{6}{c|}{\textbf{Detection Methods Based on FS}} & \multicolumn{2}{c|}{\textbf{Based on ETA}} & \multirow{2}{*}{\makecell[c]{\textbf{Ours}}} \\
             & & \textbf{FS} & \textbf{Co+FS} & \textbf{DT+FS} & \textbf{ODDS+FS} & \textbf{SMOTE+FS} & \textbf{DT+ODDS+FS} & \textbf{ETA} & \textbf{DT+ODDS+ETA} \\
            \midrule 
            \multirow{3}{*}{0\%} 
 & DoHBrw & .24 $\pm$ .07 & .24 $\pm$ .04 & .53 $\pm$ .02 & .52 $\pm$ .03 & .16 $\pm$ .00 & .30 $\pm$ .17 & .62 $\pm$ .26 & .37 $\pm$ .07 & \textbf{.74} $\pm$ .03 \\
 & IDS & .20 $\pm$ .03 & .20 $\pm$ .05 & .48 $\pm$ .02 & .47 $\pm$ .02 & .16 $\pm$ .00 & .52 $\pm$ .07 & .53 $\pm$ .28 & .37 $\pm$ .09 & \textbf{.83} $\pm$ .04 \\
 & IDS/DoH & .18 $\pm$ .01 & .20 $\pm$ .05 & .41 $\pm$ .01 & .41 $\pm$ .04 & .16 $\pm$ .00 & .33 $\pm$ .10 & .56 $\pm$ .27 & .44 $\pm$ .21 & \textbf{.69} $\pm$ .01 \\
            \midrule
            \multirow{3}{*}{10\%} 
 & DoHBrw & .44 $\pm$ .01 & .20 $\pm$ .09 & .66 $\pm$ .01 & .63 $\pm$ .06 & .17 $\pm$ .00 & .57 $\pm$ .15 & .44 $\pm$ .20 & .36 $\pm$ .17 & .58 $\pm$ .03 \\
 & IDS & .68 $\pm$ .06 & .58 $\pm$ .27 & .75 $\pm$ .09 & .73 $\pm$ .11 & .44 $\pm$ .08 & .72 $\pm$ .10 & .80 $\pm$ .17 & .75 $\pm$ .12 & .76 $\pm$ .09 \\
 & IDS/DoH & .29 $\pm$ .02 & .27 $\pm$ .05 & .54 $\pm$ .02 & .56 $\pm$ .05 & .16 $\pm$ .00 & .57 $\pm$ .05 & .39 $\pm$ .22 & .29 $\pm$ .06 & \textbf{.64} $\pm$ .01 \\
            \bottomrule
        \end{tabular}
    }
\end{table*}
